# Supplementary material for: Minimax Lower Bounds for $\mathcal{H}_\infty$-Norm Estimation
Source: arXiv:1809.10855 source file (2018-09-28)
Supplement: Supplementary file 1 [file appendix.tex]

\section*{Appendix}

\begin{algorithm}[!h]
\caption{Power Method A \cite{rojas2012analyzing}}
\label{alg:power_method_A}
Input: Normalized $u^{(1)}$.\\
\For{$t = 1$ \upshape to $N$}
{
    Perform the experiment $y^{(t)} = Gu^{(t)} + \eta^{(t)}$.\\
    Create the time-reversed $\tilde y^{(t)}$.\\
    $\mu^{(t)} = \|\tilde y^{(t)}\|_2$.\\
    $u^{(t+1)} = \tilde y^{(t)} / \mu^{(t)}$.\\
    $\hat H_t = \sqrt{\mu^{(t-1)}(u^{(t-1)})^\top \tilde y^{(t)}}.$
}
\Return $\hat H_N$.
\end{algorithm}
\vspace{-0.5cm}
\begin{algorithm}[!h]
\caption{Power Method B \cite{wahlberg2010non}}
\label{alg:power_method_B}
Input: Normalized $u^{(1)}$.\\
\For{$t = 1$ \upshape to $N/2$}
{
    Perform the experiment $y^{(t)} = Gu^{(t)} + \eta^{(t)}$.\\
    Create the time-reversed $\tilde y^{(t)}$.\\
    Perform the experiment $z^{(t)} = G\tilde y^{(t)} + \eta'^{(t)}$.\\
    Create the time-reversed $\tilde z^{(t)}$.\\
    $\hat H_t = \sqrt{|(u^{(t)})^\top\tilde z^{(t)}}|$.\\
    $u^{(t+1)} = \tilde z^{(t)}/\|\tilde z^{(t)}\|_2$.
}
\Return $\hat H_{(N/2)}$.
\end{algorithm}
\vspace{-0.5cm}
\begin{algorithm}[!h]
\caption{Weighted Thompson Sampling (WTS) \cite{muller17bandit}}
\label{alg:WTS}
Input: $M, \lambda, \sigma$, $\rho_k^1 = 1/K\; \forall\; k$, $m^0=0$, $v^0 = \lambda^2 I$.\\
\For{$t = 1$ \upshape to $N$}
{
   Input design: Create the normalized input signal $u^{(t)}$ proportional to the DFT power profile $p^t=\rho^t$.\\
   Perform the experiment $y^{(t)} = Gu^{(t)} + \eta^{(t)}$ and obtain DFT coefficients $X_k^t = Y_k^t / U_k^t$. \\
   Update the posterior for all $k$:\\
   \Indp $m_k^{t+1} = \frac{\lambda^2\sum_{\ell=1}^t p_k^\ell X_k^\ell}{\sigma^2 + \lambda^2\sum_{\ell=1}^t p_k^\ell}$. \\
   $v_k^{t+1} = \lambda^2/(1+\lambda^2/\sigma^2\sum_{\ell=1}^t p_k^\ell)$. \\
   \Indm Update the posterior $\rho^{t+1}$:\\
   \Indp Draw $s^l\sim \mathcal{N_C}(m_k^{t+1},v_k^{t+1}),\quad l=1,\ldots,M$. \\
   $\rho_k^{t+1} = \frac{1}{M}\sum_{l=1}^M \#(\argmax_i\{|s_i^l|\}=k)$. \\
   \Indm $\hat H_t = \max_k \sum_{\ell=1}^t p_k^\ell X_k^\ell / \sum_{\ell=1}^t p_k^\ell$.
}
\Return $\hat H_N$.
\end{algorithm}
